# Supplementary material for: Online Intention Prediction via Control-Informed Learning
Source: arXiv:2604.09303 source file (2026-04-10)
Supplement: Supplementary file 1 [file Supplementary.tex]

\begin{appendix}

\section{Experiment Details} \label{Appendix:experimentalDetails}
\subsection{Dynamics and Control Objective}\label{Appendix:dynamics}
\textbf{Quadrotor UAV.} We consider a quadrotor UAV with the following dynamics

\begin{equation} \label{eq:quadrotor_dyn}
    \begin{aligned} 
         \dot{\boldsymbol{p}}_I &= \boldsymbol{v}_I, \\
         m\dot{\boldsymbol{v}}_I &= m\boldsymbol{g}_I+\mathbf{F}_I, \\
         \dot{\boldsymbol{q}}_{B/I} &= \frac{1}{2}\boldsymbol{\Omega}(\boldsymbol{\omega}_B)\boldsymbol{q}_{B/I}, \\
         J_B\dot{\boldsymbol{\omega}}_B &= \mathbf{M}_B - \boldsymbol{\omega} \times J_B\boldsymbol{\omega}_B.
    \end{aligned}
\end{equation}
Here, the subscription $_B$ and $_I$ denote a quantity expressed in the body frame and inertial (world) frame, respectively; $m$ and $J_B\in\mathbb{R}^{3\times 3}$ are the mass and moment of inertia with respect to the body frame of the UAV, respectively. $g$ is the gravitational constant ($g=10\,\text{m}/\text{s}^2$), $\boldsymbol{g}_I=[0,0,g]^\prime$. $\boldsymbol{p}_I\in\mathbb{R}^3$  and $\boldsymbol{v}_I\in\mathbb{R}^3$ are the position and velocity vector of the UAV; $\boldsymbol\omega_B\in\mathbb{R}^3$ is the angular velocity vector of the UAV; $\boldsymbol{q}_{B/I}\in\mathbb{R}^4$ is the unit quaternion \cite{kuipers1999quaternions} that describes the attitude of UAV with respect to the inertial frame; $\boldsymbol{\Omega}(\boldsymbol\omega_B)$ is defined as:
\begin{equation}
    \boldsymbol{\Omega}(\boldsymbol\omega_B) =
    \begin{bmatrix}
    0&-\omega_x&-\omega_y&-\omega_z \\
    \omega_x&0&\omega_z &-\omega_y \\
    \omega_y&-\omega_z &0&\omega_x \\
    \omega_z &\omega_y&-\omega_x&0
    \end{bmatrix},
\end{equation}
$\mathbf{M}_B\in\mathbb{R}^3$ is the torque applied to the UAV; $\mathbf{F}_I\in\mathbb{R}^3$ is the force vector applied to the UAV center of mass. The total force magnitude $f=\|\mathbf{F}_I\|\in\mathbb{R}$ (along z-axis of the body frame) and torque $\mathbf{M}_B=[M_x,M_y,M_z]^\prime$ are generated by thrust from four rotating propellers $[T_1, T_2, T_3, T_4]^\prime$, their relationship can be expressed as:

\begin{equation}
    \begin{bmatrix}
    f\\
    M_x\\
    M_y\\
    M_z
    \end{bmatrix}
    =
    \begin{bmatrix}
    1&1&1&1 \\
    0&-l_w/2&0&l_w/2 \\
    -l_w/2&0&l_w/2&0 \\
    c&-c&c&-c
    \end{bmatrix}
    \begin{bmatrix}
    T_1\\
    T_2\\
    T_3\\
    T_4
    \end{bmatrix},
\end{equation}
where $l_w$ is the wing length of the UAV and $c$ is a fixed constant.
The state and input vectors of the UAV are defined as:
\begin{equation}
    \begin{aligned}
        \boldsymbol{x} &\triangleq
        \begin{bmatrix}
        \boldsymbol{p}_I'& \boldsymbol{v}_I'& \boldsymbol{q}_{B/I}' & \boldsymbol\omega_B'
        \end{bmatrix}
        ' \in \mathbb{R}^{13}, \\
        \boldsymbol{u} &\triangleq
        \begin{bmatrix}
        T_1&T_2&T_3&T_4
        \end{bmatrix}
        '\in\mathbb{R}^4.
    \end{aligned}
\end{equation}
The runnning cost and final cost are 
\begin{equation}
\begin{split}
\boldsymbol{\omega}_{\mathrm{r}}^{\prime} c_{\mathrm{r}}(\boldsymbol{x}_t,\boldsymbol{u}_t,\boldsymbol{x}_{\mathrm{g}})  = \ &\boldsymbol{\omega}_{\mathrm{r}}^{\prime}||\boldsymbol{u}_t||^2 \\
\boldsymbol{\omega}_{\mathrm{f}}^{\prime} c_{\mathrm{f}}(\boldsymbol{x}_T,\boldsymbol{x}_{\mathrm{g}}) = \ &\boldsymbol{\omega}_{\mathrm{f},\boldsymbol{p}}^{\prime}||\boldsymbol{x}_T[1:3]-\boldsymbol{x}_{\mathrm{g}}[1:3]||^2 + \\
& \boldsymbol{\omega}_{\mathrm{f},\boldsymbol{v}}^{\prime}||\boldsymbol{x}_T[4:6]-\boldsymbol{x}_{\mathrm{g}}[4:6]||^2 + \\
& \boldsymbol{\omega}_{\mathrm{f},\boldsymbol{q}}^{\prime}||\boldsymbol{x}_T[7:10]-\boldsymbol{x}_{\mathrm{g}}[7:10]||^2 + \\
& \boldsymbol{\omega}_{\mathrm{f},\boldsymbol{\omega}}^{\prime}||\boldsymbol{x}_T[11:13]-\boldsymbol{x}_{\mathrm{g}}[11:13]||^2.
\end{split}
\end{equation}
Here, $\boldsymbol{\omega}_{\mathrm{f}} = \begin{bmatrix}
    \boldsymbol{\omega}_{\mathrm{f},\boldsymbol{p}}^{\prime} & \boldsymbol{\omega}_{\mathrm{f},\boldsymbol{v}}^{\prime} & \boldsymbol{\omega}_{\mathrm{f},\boldsymbol{q}}^{\prime} & \boldsymbol{\omega}_{\mathrm{f},\boldsymbol{\omega}}^{\prime}
\end{bmatrix}^{\prime}$.
The parameters used for UAV experiments are summarized in Table~\ref{table:quadrotor_para}.
The true parameter is $\boldsymbol{\theta}^* = [1,1,1,1,0.4,0.01,0.1,10,1,5,1,\boldsymbol{x}_{\mathrm{g}}^{*\prime}]
^\prime
\in\mathbb{R}^{24}$, where $\boldsymbol{x}_{\mathrm{g}}^{*\prime}$ is randomly generated for each case.
% \begin{center}
% \begin{tabular}{ | c | c | c | c | } 
%   \hline
%   Dynamics Parameters & Values & Objective Parameters & Values \\
%   \hline
%     $J_{B}$ & $\boldsymbol{I}_3$ kg$\cdot$m$^2$ & $\boldsymbol{\omega}_{\mathrm{r}}$  & 0.1 \\ 
%   \hline
%     $m$ & $1$ kg & $\boldsymbol{\omega}_{\mathrm{f},\boldsymbol{p}}$  & 10 \\ 
%   \hline
%     $l_w$ & $0.4$ m & $\boldsymbol{\omega}_{\mathrm{f},\boldsymbol{v}}$  & 1 \\ 
%   \hline
%     $c$ & $0.01$ m & $\boldsymbol{\omega}_{\mathrm{f},\boldsymbol{q}}$  & 5 \\ 
%   \hline
%      &  & $\boldsymbol{\omega}_{\mathrm{f},\boldsymbol{\omega}}$  & 1 \\ 
%   \hline
% \end{tabular}
% \end{center}

\begin{table}
\centering
\begin{threeparttable}
\caption{UAV Parameters} \label{table:quadrotor_para}
\begin{tabular}{c | c | c | c}
\toprule
Dynamics Parameter & Value & Objective Parameter & Value \\
\midrule
$J_{B}$ & $\boldsymbol{I}_3$ kg$\cdot$m$^2$ & $\boldsymbol{\omega}_{\mathrm{r}}$  & 0.1 \\
$m$ & $1$ kg & $\boldsymbol{\omega}_{\mathrm{f},\boldsymbol{p}}$  & 10 \\
$l_w$ & $0.4$ m & $\boldsymbol{\omega}_{\mathrm{f},\boldsymbol{v}}$  & 1 \\
$c$ & $0.01$ m & $\boldsymbol{\omega}_{\mathrm{f},\boldsymbol{q}}$  & 5 \\
 &  & $\boldsymbol{\omega}_{\mathrm{f},\boldsymbol{\omega}}$  & 1 \\ 
\bottomrule
\end{tabular}
\end{threeparttable}
\centering
\end{table}

\subsection{Hyperparameter Settings} 
\label{appendix:hyperparameter}
\textbf{Partially Known Dynamics.} In section \ref{sec:exp}, the initial guess for the dynamics and objective parameters are randomized within a range of $\pm25\%$ around the true parameters. We add a lower bound of $10^{-8}$ for the dynamics and objective parameters. The UAV's initial state is used as the guess for the goal state.
For an arbitrary row vector $\boldsymbol{v} \in \mathbb{R}^{1\times s}$ or column vector $\boldsymbol{v} \in \mathbb{R}^s$, denote $\text{diag}([\boldsymbol{v}]) \in \mathbb{R}^{s\times s}$ as a diagonal matrix with its diagonal elements are the elements of $\boldsymbol{v}$.
The initial parameters of Real-time Intention Predictor \eqref{eq:EKF} for each case are summarized in Table~\ref{table:mat_partial}.
\begin{table}
\centering
\begin{threeparttable}
\caption{Initial Parameters of Real-time Intention Predictor  with Partially Known Dynamics} \label{table:mat_partial}
\begin{tabular}{c | c | c | c}
\toprule
Noise Type & $\sigma$ & $\boldsymbol{P}_{-1}$ & $\boldsymbol{R}_{-1}$ \\
\midrule
No Noise & 0 & diag([$10^{-7}\cdot\boldsymbol{1}_{1\times 11}$,$\ 10^{-4}\cdot\boldsymbol{1}_{1\times 3}$,$\ 10^{-7}\cdot\boldsymbol{1}_{1\times 10}$]) &diag([$10^{-9}\cdot\boldsymbol{1}_{1\times 13}$]) \\
Uniform & 0.1 & diag([$10^{-8}\cdot\boldsymbol{1}_{1\times 11}$,$\ 10^{-4}\cdot\boldsymbol{1}_{1\times 3}$,$10^{-8}\cdot\boldsymbol{1}_{1\times 10}$]) & diag([$10^{-7}\cdot\boldsymbol{1}_{1\times 13}$]) \\
Uniform & 0.5 & diag([$10^{-9}\cdot\boldsymbol{1}_{1\times 11}$,$\ 10^{-5}\cdot\boldsymbol{1}_{1\times 3}$,$\ 10^{-9}\cdot\boldsymbol{1}_{1\times 10}$]) & diag([$10^{-7}\cdot\boldsymbol{1}_{1\times 13}$]) \\
Uniform & 1 & diag([$10^{-11}\cdot\boldsymbol{1}_{1\times 11}$,$\ 10^{-6}\cdot\boldsymbol{1}_{1\times 3}$,$\ 10^{-11}\cdot\boldsymbol{1}_{1\times 10}$]) & diag([$10^{-7}\cdot\boldsymbol{1}_{1\times 13}$]) \\
Gaussian & 0.1 & diag([$10^{-8}\cdot\boldsymbol{1}_{1\times 11}$,$\ 10^{-4}\cdot\boldsymbol{1}_{1\times 3}$,$\ 10^{-8}\cdot\boldsymbol{1}_{1\times 10}$]) & diag([$10^{-7}\cdot\boldsymbol{1}_{1\times 13}$]) \\
Gaussian & 0.5 & diag([$10^{-9}\cdot\boldsymbol{1}_{1\times 11}$,$\ 10^{-5}\cdot\boldsymbol{1}_{1\times 3}$,$10^{-9}\cdot\boldsymbol{1}_{1\times 10}$]) & diag([$10^{-7}\cdot\boldsymbol{1}_{1\times 13}$]) \\
Gaussian & 1 & diag([$10^{-11}\cdot\boldsymbol{1}_{1\times 11}$,$\ 10^{-6}\cdot\boldsymbol{1}_{1\times 3}$,$\ 10^{-11}\cdot\boldsymbol{1}_{1\times 10}$]) & diag([$10^{-7}\cdot\boldsymbol{1}_{1\times 13}$]) \\
\bottomrule
\end{tabular}
\end{threeparttable}
\centering
\end{table}
\textbf{Unknown Dynamics (Neural Dynamics).} In section \ref{sec:nn}, the dynamics of the UAV is a neural network and the other setup remains the same as section \ref{sec:exp}. The size of three neural networks are: $4(n+m) \times n$ with 2121 parameters; $2(n+m)\times 4(n+m) \times n$ with 3889 parameters; and $2(n+m)\times 4(n+m) \times 2(n+m)\times n$ with 5793 parameters. The measurement noise is a multivariate Gaussian distribution with $\sigma=0.5$. The running cost is assumed to be 0.1. The initial guess for the neural dynamics is randomly generated and objective parameters are randomized within a range of $\pm0.25$ around the true parameters.
The initial parameters of Real-time Intention Predictor \eqref{eq:EKF} are summarized in Table~\ref{table:mat_unknown}.
% \begin{center}
% \begin{tabular}{ | c | c | c | c | } 
%   \hline
%   Noise Type & $\sigma$ & $\boldsymbol{P}_0$ & $\boldsymbol{R}_0$ \\
%   \hline
%   Gaussian & 0.5 & diag([$10^{-8}\cdot\boldsymbol{1}_{1\times 3893}$,$\ 10^{-5}\cdot\boldsymbol{1}_{1\times 3}$,$\ 10^{-8}\cdot\boldsymbol{1}_{1\times 10}$]) & diag([$10^{-8}\cdot\boldsymbol{1}_{1\times 13}$]) \\
%   \hline
% \end{tabular}
% \end{center}

\begin{table}
\centering
\begin{threeparttable}
\caption{Initial Parameters of Real-time Intention Predictor  with Unknown Known Dynamics} \label{table:mat_unknown}
\begin{tabular}{c | c | c}
\toprule
NN Parameter Size & $\boldsymbol{P}_{-1}$ & $\boldsymbol{R}_{-1}$ \\
\midrule
2121 & diag([$10^{-8}\cdot\boldsymbol{1}_{1\times 2125}$,$\ 10^{-5}\cdot\boldsymbol{1}_{1\times 3}$,$\ 10^{-8}\cdot\boldsymbol{1}_{1\times 10}$]) & diag([$10^{-8}\cdot\boldsymbol{1}_{1\times 13}$]) \\
\midrule
3889 & diag([$10^{-8}\cdot\boldsymbol{1}_{1\times 3893}$,$\ 10^{-5}\cdot\boldsymbol{1}_{1\times 3}$,$\ 10^{-8}\cdot\boldsymbol{1}_{1\times 10}$]) & diag([$10^{-8}\cdot\boldsymbol{1}_{1\times 13}$]) \\
\midrule
5793 & diag([$10^{-8}\cdot\boldsymbol{1}_{1\times 5797}$,$\ 10^{-5}\cdot\boldsymbol{1}_{1\times 3}$,$\ 10^{-8}\cdot\boldsymbol{1}_{1\times 10}$]) & diag([$10^{-8}\cdot\boldsymbol{1}_{1\times 13}$]) \\
\bottomrule
\end{tabular}
\end{threeparttable}
\centering
\end{table}

\end{appendix}
